# Supplementary material for: Non-Smooth Setting of Stochastic Decentralized Convex Optimization Problem Over Time-Varying Graphs
Source: arXiv:2307.00392 source file (2023-09-05)
Supplement: Supplementary file 1 [file 5_Appendix.tex]

\section{Proof of Theorem \ref{th:ZOSADOM_aw}} \label{proof_Theorem2_aw}
\subsection{Smooth approximation}\label{Subsection:smoothing_approximation}
    Since problem \eqref{eq:nonsmooth_init_problem_aw} is non-smooth, we introduce a smooth approximation of the non-smooth function $F$ as follows:
    \begin{equation}\label{f_gamma}
        F_\gamma(x) := \mathbb{E}_{\tilde{e}} \left[ F(x + \gamma \tilde{e}) \right],
    \end{equation}
    where $\gamma > 0$ is smoothing parameter, $\tilde{e}$ is random vector uniformly distributed on $B_2^d(\gamma)$. The following lemma provides the connection between non-smooth function $F$ and smoothed function $F_\gamma$.
    
    \begin{lemma}\label{Lemma:connect_f_with_f_gamma}
        Let Assumptions \ref{ass:Lipschitz_continuity_aw}, \ref{ass:convexity_Q_gamma} it holds, then for all $x \in Q$ we have
        \begin{equation*}
            F(x)\leq F_\gamma(x) \leq F(x) + \gamma M_2.
        \end{equation*}
    \end{lemma}
    \begin{proof}
    For the first inequality we use the convexity of the function $F(x)$
    \begin{equation*}
        F_\gamma(x) = \mathbb{E}_{\Tilde{e}} \left[ F(x + \gamma \Tilde{e}) \right] \geq \mathbb{E}_{\Tilde{e}} \left[ F(x) + \dotprod{\nabla F(x)}{\gamma \Tilde{e}}) \right] = \mathbb{E}_{\Tilde{e}} \left[ F(x) \right] = F(x).
    \end{equation*}
    For the second inequality we have
    \begin{eqnarray*}
        | F_\gamma (x)- F(x) | = | \mathbb{E}_{\Tilde{e}} \left[ F(x + \gamma \Tilde{e}) \right] - F(x) | &\leq& \mathbb{E}_{\Tilde{e}} \left[ | F(x + \gamma \Tilde{e}) - F(x) | \right]\\
        &\leq& \gamma M_2 \mathbb{E}_{\Tilde{e}} \left[ \| \Tilde{e} \| \right] \leq \gamma M_2,
    \end{eqnarray*}
    using the fact that $F$ is $M_2$-Lipschitz function.
    \end{proof}
    
    The next lemmas provide properties of the smoothed function $F_\gamma$.
    \begin{lemma}\label{Lemma:M_lipschitz_continuity}
        Let Assumptions \ref{ass:Lipschitz_continuity}, \ref{ass:convexity_Q_gamma} it holds, then for $F_\gamma(x)$ from \eqref{f_gamma} we have
        \begin{equation*}
            |F_\gamma(y) - F_\gamma(x) | \leq M_2 \| y - x \|, \;\;\; \forall x,y \in Q.
        \end{equation*}
    \end{lemma}
    \begin{proof} Using $M_2$-Lipschitz continuity of function $f$ we obtain
        \begin{eqnarray*}
            | F_\gamma (y)- F_\gamma(x) | \leq \mathbb{E}_{\Tilde{e}} \left[ | f(y + \gamma \Tilde{e})  - F(x + \gamma \Tilde{e}) | \right] \leq M_2 \| y - x \|.
        \end{eqnarray*}
    \end{proof}
    
    %\newpage%%%%%%%%%%%%%%%%%%%%%%%%%%%%%%%%%%%%%%%%%
    
    \begin{lemma}[Theorem 1, \cite{Gasnikov_ICML}]\label{Lemma:Lipschitz_gradient}
        Let Assumptions \ref{ass:Lipschitz_continuity}, \ref{ass:convexity_Q_gamma} it holds, then $F_\gamma(x)$ has $L_{F_\gamma} = \frac{\sqrt{d}M_2}{\gamma}$-Lipschitz gradient
        \begin{equation*}
            \| \nabla F_\gamma(y) - \nabla F_\gamma(x) \| \leq L_{f_{\gamma}} \| y - x \|, \;\;\; \forall x,y \in Q.
        \end{equation*}
    \end{lemma}
    
    \subsection{Gradient via $l_2$ randomization}\label{Subsection:l2_randomization}
    The gradient of $F_\gamma(x,\xi)$ can be estimated by the following approximation:
    \begin{equation}
        \nabla F_\gamma(x, \xi, e) = \frac{d}{2 \gamma} \left( F_\delta(x+ \gamma e, \xi) - F_\delta(x - \gamma e, \xi) \right) e,
    \end{equation}
    where $F_\delta(x,\xi)$ is gradient-free oracle from Definition \ref{def:GFOracle}, $e$ is a random vector uniformly distributed on $S_2^d(\gamma)$. The following lemma provides properties of the gradient $\nabla F_\gamma(x,\xi,e)$.
    
    \begin{lemma}[Lemma 2, \cite{Lobanov_2022}]\label{Lemma:sigma}
         Gradient $\nabla F_\gamma(x,\xi,e)$ has bounded variance (second moment) for all $x \in Q$
        \begin{equation*}
           \mathbb{E}_{\xi, e} \left[ \| \nabla F_\gamma (x, \xi, e) \|^2 \right] \leq 2 \sqrt{2} \left( d M_2^2 + \frac{d^2 \Delta^2}{\sqrt{2} \gamma^2}  \right). 
        \end{equation*}
    \end{lemma}
    \begin{remark}\label{Remark:sigma}
        Using the fact that the second moment is the upper estimate of the variance for the unbiased gradient and assuming that $\Delta$ is sufficiently small we obtain the following estimate of the variance from Lemma \ref{Lemma:sigma}:
        \begin{equation*}
            \sigma^2 \leq 4 \sqrt{2} d M_2^2.
        \end{equation*}
    \end{remark}
    \begin{proof}[Proof of Theorem \ref{th:ZOSADOM}]
        Write out the convergence rate of the SADOM algorithm:
        \begin{align*}
	\expect{\sqn{x^N - x^*}} &\leq \eta\expect{\Psi_x^N} \leq \eta (\expect{\Psi_x^N} + \expect{\Psi_{yz}^N} ) \leq \left(1 - \frac{\lmin\sqrt{\mu}}{32\lmax\sqrt{L}}\right)^N\eta(\Psi_x^0 + \Psi_{yz}^0) + 32 \chi \frac{\eta \sigma^2}{\mu B}.
	\end{align*}
	Choosing $C = \eta(\Psi_x^0 + \Psi_{yz}^0)$ and substituting $\sigma^2 \leq 2 \sqrt{2} \min \left\{ q, \ln d \right\} d^{2 - \frac{2}{p}}  M_2^2$, and $L_{F_\gamma} = \frac{\sqrt{d}M}{\gamma}$, and  \al{$\eta = (\sqrt{\mu L})^{-1}$}, and using $\gamma = \frac{\varepsilon}{2 M_2}$, \al{we get $\expect{\sqn{x^N - x^*}} \leq \epsilon$} after
	\begin{equation*}
	N_{\text{comm}} = 32\chi\sqrt{\frac{L}{\mu}}\log \frac{C}{\varepsilon} = \mathcal{O} \left( \chi\sqrt{\frac{L}{\mu}}\log \frac{1}{\epsilon}\right) = \mathcal{O} \left( \chi\frac{d^{1/4} \sqrt{M M_2}}{\sqrt{\varepsilon \mu}}\log \frac{1}{\epsilon}\right)
	\end{equation*}
       number of communication rounds and 
        \begin{equation*}
            T = N \cdot B = \tilde{\mathcal{O}}\left( \frac{\sigma^2}{\mu^2 \epsilon} \right) = \tilde{\mathcal{O}}\left( \frac{ d M_2^2}{\mu^2 \epsilon} \right)
        \end{equation*}
	oracle calls per node, \al{where $\varepsilon$-accuracy: $\expect{f(x^N) - f(x^*)} \leq \varepsilon$}.
    \end{proof}
